# Supplementary material for: Robustness Evaluation of Entity Disambiguation Using Prior Probes:the Case of Entity Overshadowing
Source: arXiv:2108.10949 source file (2021-12-14)
Supplement: Supplementary file 1 [file _7_appendix.tex]

% \newpage
\section{Additional quality assurance}
\label{sec:appendix}

Table~\ref{tbl:mini-benchmark} shows the evaluation results of all baselines on the manually controlled subset of ShadowLink, which consists of 37 top-entities and 37 shadow-entities. This serves as an additional quality assurance step: the scores of all systems remain considerably lower than their respective scores on the $Tail$ subset (see Table~\ref{tbl:res-all}), which proves that the main challenge is caused by entity overshadowing and not by the quality of the textual examples.
% Maybe write smth about tagme
\begin{table*}[h!]
\centering
\begin{tabular}{@{}lllllll@{}}
\toprule
\multicolumn{1}{c}{\multirow{2}{*}{Baseline}} & \multicolumn{3}{c}{\textbf{Shadow-mini}} & \multicolumn{3}{c}{\textbf{Top-mini}} \\ \cmidrule(l){2-7} 
\multicolumn{1}{c}{} & F & P & R & F & P & R \\ \midrule
AGDISTIS/MAG & 0.275 & 0.275 & \multicolumn{1}{l|}{0.275} & 0.297 & 0.297 & 0.297 \\
AIDA & 0.328 & 0.407 & \multicolumn{1}{l|}{0.275} & 0.387 & 0.480 & 0.324 \\
DBpedia Spotlight & 0.121 & 0.154 & \multicolumn{1}{l|}{0.100} & 0.393 & 0.500 & 0.324 \\
FOX & 0.070 & 0.118 & \multicolumn{1}{l|}{0.050} & 0.200 & 0.385 & 0.135 \\
GENRE & 0.500 & 0.500 & \multicolumn{1}{l|}{0.500} & 0.543 & 0.543 & 0.543 \\
REL & 0.235 & 0.235 & \multicolumn{1}{l|}{0.235} & 0.600 & 0.600 & 0.600 \\
TagMe 2 & 0.563 & 0.750 & \multicolumn{1}{l|}{0.450} & 0.529 & 0.581 & 0.487 \\
WAT & 0.280 & 0.700 & 0.175 & 0.548 & 0.680 & 0.460 \\ \bottomrule
\end{tabular}
\caption{\label{tbl:mini-benchmark} Benchmark evaluation results on the manually controlled sample}
\end{table*}
